# Supplementary material for: The GALAH+ Survey: Third Data Release
Source: arXiv:2011.02505 source file (2021-04-28)
Supplement: Supplementary file 1 [file GALAH_DR3_abundances_lines.tex]

Elem. & $\lambda$ [$\mathrm{\AA}$] & LEP [eV] & $\log(gf)$ & Ref. & Mask & Segment\\
\hline
Li1 & 6707.7635 & 0.000 & -0.002 & (1) & 6707.30-6708.30 & 6705.76-6709.76\\
Li1 & 6707.7635 & 0.000 & -0.002 & (1) & 6707.30-6708.30 & 6705.76-6709.76\\
C 1 & 6587.6100 & 8.537 & -1.021 & (2) & 6587.26-6587.99 & 6585.61-6589.61\\
O 1 & 7771.9440 & 9.146 & 0.369 & (3) & 7771.36-7772.51 & 7769.50-7777.50\\
O 1 & 7774.1660 & 9.146 & 0.223 & (3) & 7773.52-7774.78 & 7769.50-7777.50\\
O 1 & 7775.3880 & 9.146 & 0.002 & (3) & 7774.91-7775.96 & 7769.50-7777.50\\
Na1 & 5682.6333 & 2.102 & -0.706 & (4) & 5682.52-5683.00 & 5680.63-5691.20\\
Na1 & 5688.2050 & 2.104 & -0.404 & (4) & 5687.92-5688.39 & 5680.63-5691.20\\
Mg1 & 5711.0880 & 4.346 & -1.842 & (5) & 5710.76-5711.43 & 5710.00-5713.09\\
Al1 & 6696.0230 & 3.143 & -1.569 & (6) & 6695.78-6696.17 & 6695.00-6699.87\\
Al1 & 6698.6730 & 3.143 & -1.870 & (6) & 6698.39-6698.90 & 6695.00-6699.87\\
Al1 & 7835.3090 & 4.022 & -0.689 & (7) & 7834.88-7835.57 & 7834.00-7837.50\\
Al1 & 7836.1340 & 4.022 & -1.795 & (8) & 7835.81-7836.43 & 7834.00-7837.50\\
Al1 & 7836.1340 & 4.022 & -0.534 & (7) & 7835.81-7836.43 & 7834.00-7837.50\\
Si1 & 5684.4840 & 4.954 & -1.553 & (9) & 5684.18-5684.78 & 5683.00-5686.00\\
Si1 & 5690.4250 & 4.930 & -1.773 & (9) & 5690.18-5690.68 & 5688.43-5692.43\\
Si1 & 5701.1040 & 4.930 & -1.953 & (9) & 5700.93-5701.29 & 5699.70-5702.00\\
Si1 & 5772.1460 & 5.082 & -1.653 & (9) & 5771.85-5772.45 & 5771.15-5773.15\\
Si1 & 5793.0726 & 4.930 & -1.963 & (9) & 5792.72-5793.39 & 5791.07-5794.70\\
Si1 & 6721.8481 & 5.863 & -1.062 & (10) & 6721.20-6722.30 & 6718.45-6723.85\\
Si1 & 7680.2660 & 5.863 & -0.590 & (9) & 7679.94-7680.67 & 7678.27-7682.27\\
K 1 & 7698.9643 & 0.000 & -0.176 & (11) & 7698.57-7699.30 & 7696.96-7700.96\\
Ca1 & 5857.4510 & 2.933 & 0.240 & (12) & 5857.02-5857.62 & 5855.45-5859.45\\
Ca1 & 5867.5620 & 2.933 & -1.570 & (12) & 5867.30-5867.70 & 5865.50-5869.80\\
Ca1 & 6493.7810 & 2.521 & -0.109 & (13) & 6493.47-6493.99 & 6491.78-6501.65\\
Ca1 & 6499.6500 & 2.523 & -0.818 & (13) & 6499.38-6499.95 & 6491.78-6501.65\\
Sc1 & 4743.8300 & 1.448 & 0.422 & (14) & 4743.55-4744.00 & 4741.83-4746.83\\
Sc1 & 4753.1610 & 0.000 & -1.659 & (14) & 4753.00-4753.40 & 4751.30-4755.50\\
Sc2 & 5657.8960 & 1.507 & -0.603 & (14) & 5657.68-5658.12 & 5655.90-5659.90\\
Sc2 & 5667.1490 & 1.500 & -1.309 & (14) & 5666.91-5667.32 & 5665.15-5669.15\\
Sc1 & 5671.8163 & 1.448 & -0.290 & (14) & 5671.60-5672.09 & 5669.82-5673.82\\
Sc1 & 5717.3070 & 1.440 & -0.532 & (14) & 5717.00-5717.50 & 5715.50-5719.50\\
Sc1 & 5724.1070 & 1.433 & -0.661 & (14) & 5723.89-5724.27 & 5722.11-5726.11\\
Sc2 & 6604.6010 & 1.357 & -1.309 & (14) & 6604.41-6604.98 & 6602.60-6606.60\\
Ti1 & 4758.1178 & 2.249 & 0.510 & (15) & 4757.95-4758.31 & 4756.12-4760.12\\
Ti1 & 4759.2697 & 2.256 & 0.590 & (15) & 4759.09-4759.49 & 4756.12-4760.12\\
Ti1 & 4778.2547 & 2.236 & -0.350 & (15) & 4778.08-4778.44 & 4776.25-4780.00\\
Ti1 & 4781.7106 & 0.848 & -1.950 & (16) & 4781.57-4781.93 & 4780.50-4782.76\\
Ti1 & 4797.9757 & 2.334 & -0.630 & (16) & 4797.84-4798.13 & 4796.33-4799.41\\
Ti1 & 4801.9016 & 0.818 & -3.060 & (16) & 4801.80-4802.20 & 4800.00-4803.90\\
Ti1 & 4820.4094 & 1.503 & -0.380 & (15) & 4820.09-4820.67 & 4818.41-4822.41\\
Ti1 & 5689.4600 & 2.297 & -0.360 & (17) & 5689.26-5689.81 & 5687.46-5691.46\\
Ti1 & 5716.4500 & 2.297 & -0.720 & (17) & 5716.23-5716.83 & 5714.45-5718.45\\
Ti1 & 5716.4500 & 0.871 & -0.258 & (18) & 5716.23-5716.83 & 5714.45-5718.45\\
Ti1 & 5716.4500 & 1.511 & 0.895 & (18) & 5716.23-5716.83 & 5714.45-5718.45\\
Ti1 & 5720.4359 & 2.292 & -0.900 & (19) & 5720.24-5720.68 & 5718.50-5722.50\\
Ti1 & 5739.4690 & 2.249 & -0.610 & (15) & 5739.25-5739.70 & 5737.47-5741.47\\
Ti1 & 5866.4513 & 1.067 & -0.790 & (15) & 5866.00-5866.81 & 5864.78-5868.60\\
Ti1 & 6599.1080 & 0.887 & 0.633 & (18) & 6598.90-6599.50 & 6597.11-6601.11\\
Ti1 & 6716.6660 & 2.488 & -1.370 & (16) & 6716.49-6716.90 & 6714.67-6718.67\\
Ti1 & 7852.6770 & 0.848 & -2.640 & (20) & 7852.20-7853.00 & 7851.36-7854.67\\
Ti2 & 4719.5109 & 1.243 & -3.320 & (21) & 4719.30-4719.60 & 4719.00-4721.51\\
Ti2 & 4764.5247 & 1.237 & -2.690 & (22) & 4764.40-4764.80 & 4762.52-4766.52\\
Ti2 & 4798.5313 & 1.080 & -2.660 & (22) & 4798.33-4798.64 & 4796.33-4799.41\\
Ti2 & 4849.1678 & 1.131 & -2.960 & (21) & 4849.05-4849.40 & 4847.17-4851.17\\
Ti2 & 4865.6104 & 1.116 & -2.700 & (22) & 4865.30-4865.85 & 4863.61-4867.61\\
Ti2 & 4874.0094 & 3.095 & -0.860 & (22) & 4873.87-4874.19 & 4872.01-4876.01\\
V 1 & 4831.6457 & 0.017 & -1.380 & (19) & 4831.52-4831.73 & 4829.65-4833.65\\
V 1 & 4784.4665 & 0.017 & -2.670 & (19) & 4784.34-4784.61 & 4782.47-4786.47\\
V 1 & 4796.9140 & 2.097 & 0.190 & (23) & 4796.76-4796.98 & 4794.91-4798.91\\
Cr1 & 4775.1300 & 3.551 & -1.050 & (19) & 4774.95-4775.31 & 4773.13-4777.13\\
Cr1 & 4789.3350 & 2.544 & -0.330 & (24) & 4789.19-4789.48 & 4787.34-4791.34\\
Cr1 & 4801.0247 & 3.122 & -0.131 & (19) & 4800.84-4801.23 & 4799.02-4803.02\\
Cr1 & 5787.9190 & 3.322 & -0.083 & (19) & 5787.64-5788.16 & 5786.32-5790.42\\
Cr1 & 6630.0100 & 1.030 & -3.560 & (19) & 6629.77-6630.27 & 6627.51-6632.51\\
Mn1 & 4739.0900 & 2.941 & -0.604 & (25) & 4738.90-4739.30 & 4737.09-4741.09\\
Mn1 & 4754.0301 & 2.282 & -0.787 & (25) & 4753.80-4754.30 & 4752.04-4755.60\\
Mn1 & 4761.5060 & 2.953 & -0.548 & (25) & 4761.35-4761.76 & 4759.51-4763.51\\
Co1 & 4781.4283 & 1.883 & -2.150 & (26) & 4781.13-4781.73 & 4779.43-4783.43\\
Co1 & 4899.5135 & 2.042 & -1.597 & (27) & 4899.21-4899.81 & 4897.51-4901.51\\
Co1 & 6551.4491 & 1.883 & -2.645 & (27) & 6551.15-6551.75 & 6549.45-6553.45\\
Co1 & 6632.4505 & 2.280 & -2.726 & (28) & 6632.22-6632.78 & 6630.45-6634.45\\
Co1 & 6678.8091 & 1.956 & -2.680 & (26) & 6678.51-6679.11 & 6676.81-6680.81\\
Co1 & 7712.6628 & 2.542 & -1.570 & (26) & 7712.44-7713.05 & 7710.66-7714.66\\
Co1 & 7838.1261 & 3.971 & -0.300 & (26) & 7837.79-7838.50 & 7836.13-7840.13\\
Ni1 & 5846.9935 & 1.676 & -3.460 & (29) & 5846.80-5847.21 & 5844.99-5848.99\\
Ni1 & 6586.3098 & 1.951 & -2.780 & (29) & 6586.00-6586.48 & 6584.31-6588.31\\
Cu1 & 5700.2326 & 1.642 & -2.978 & (30) & 5699.94-5700.39 & 5698.23-5702.23\\
Cu1 & 5782.1554 & 1.642 & -2.148 & (30) & 5781.90-5782.47 & 5780.16-5784.16\\
Zn1 & 4722.1530 & 4.030 & -0.380 & (31) & 4721.71-4722.40 & 4721.15-4725.15\\
Zn1 & 4810.5280 & 4.078 & -0.160 & (32) & 4810.30-4810.75 & 4806.53-4814.53\\
Rb1 & 7800.2590 & 0.000 & 0.144 & (31) & 7800.14-7800.47 & 7798.26-7802.26\\
Sr1 & 6550.2440 & 2.690 & 0.460 & (33) & 6550.09-6550.44 & 6548.24-6552.24\\
Y 1 & 4819.6383 & 1.356 & -0.462 & (34) & 4819.34-4819.94 & 4817.64-4821.64\\
Y 2 & 4854.8611 & 0.992 & -0.270 & (35) & 4854.62-4855.10 & 4852.86-4856.86\\
Y 2 & 4883.6821 & 1.084 & 0.190 & (35) & 4883.45-4883.90 & 4881.68-4885.68\\
Y 2 & 5662.9241 & 1.944 & 0.340 & (35) & 5662.73-5663.17 & 5660.93-5664.93\\
Y 2 & 5728.8865 & 1.839 & -1.150 & (35) & 5728.73-5729.02 & 5726.89-5730.89\\
Y 1 & 4819.6383 & 1.356 & -0.462 & (34) & 4819.34-4819.94 & 4817.64-4821.64\\
Y 2 & 4854.8611 & 0.992 & -0.270 & (35) & 4854.62-4855.10 & 4852.86-4856.86\\
Y 2 & 4883.6821 & 1.084 & 0.190 & (35) & 4883.45-4883.90 & 4881.68-4885.68\\
Y 2 & 5662.9241 & 1.944 & 0.340 & (35) & 5662.73-5663.17 & 5660.93-5664.93\\
Y 2 & 5728.8865 & 1.839 & -1.150 & (35) & 5728.73-5729.02 & 5726.89-5730.89\\
Zr1 & 4739.4800 & 0.651 & 0.230 & (36) & 4739.32-4739.57 & 4737.48-4741.48\\
Zr1 & 4772.3100 & 0.623 & 0.040 & (36) & 4772.23-4772.43 & 4770.31-4774.31\\
Zr1 & 4805.8700 & 0.687 & -0.420 & (36) & 4805.72-4806.06 & 4803.87-4807.87\\
Zr1 & 4828.0400 & 0.623 & -0.640 & (36) & 4827.91-4828.20 & 4826.04-4830.04\\
Zr1 & 5680.9000 & 0.543 & -1.700 & (37) & 5680.60-5681.20 & 5678.90-5682.90\\
Mo1 & 5689.1460 & 1.382 & -1.002 & (38) & 5688.85-5689.45 & 5687.15-5691.15\\
Mo1 & 5751.4080 & 1.420 & -1.014 & (38) & 5751.30-5751.60 & 5750.30-5752.60\\
Mo1 & 5858.2660 & 1.470 & -0.996 & (38) & 5858.10-5858.50 & 5857.10-5859.50\\
Mo1 & 6619.1340 & 1.335 & -1.252 & (38) & 6618.83-6619.43 & 6617.13-6621.13\\
Ru1 & 4757.8480 & 0.928 & -0.960 & (39) & 4757.54-4758.14 & 4755.84-4759.84\\
Ru1 & 4869.1530 & 0.928 & -0.830 & (39) & 4869.03-4869.28 & 4867.15-4871.15\\
Ru1 & 5699.0560 & 1.087 & -1.470 & (39) & 5698.76-5699.36 & 5697.06-5701.06\\
Ba2 & 5853.6680 & 0.604 & -0.907 & (40) & 5853.50-5854.00 & 5851.67-5855.67\\
Ba2 & 6496.8970 & 0.604 & -0.407 & (40) & 6496.70-6497.28 & 6494.90-6498.50\\
La2 & 4716.4400 & 0.772 & -1.210 & (41) & 4716.30-4716.59 & 4712.44-4720.44\\
La2 & 4748.7300 & 0.927 & -0.540 & (41) & 4748.57-4748.92 & 4743.03-4751.73\\
La2 & 4804.0690 & 0.235 & -1.870 & (41) & 4803.85-4804.29 & 4800.04-4808.04\\
La2 & 5805.7700 & 0.126 & -1.560 & (41) & 5805.53-5805.93 & 5802.77-5809.07\\
Ce2 & 4773.9410 & 0.924 & -0.390 & (42) & 4773.84-4774.07 & 4771.94-4775.94\\
Nd2 & 4811.3420 & 0.064 & -1.140 & (43) & 4811.20-4811.53 & 4809.34-4813.34\\
Nd2 & 5740.8580 & 1.160 & -0.530 & (44) & 5740.70-5741.03 & 5738.86-5742.86\\
Nd2 & 5770.4890 & 1.081 & -1.030 & (43) & 5770.31-5770.71 & 5768.49-5772.49\\
Nd2 & 5811.5700 & 0.859 & -0.860 & (44) & 5811.34-5811.76 & 5809.57-5813.57\\
Nd2 & 5842.3660 & 1.282 & -0.600 & (43) & 5842.19-5842.62 & 5840.37-5844.37\\
Sm2 & 4719.8400 & 0.040 & -1.240 & (45) & 4719.54-4720.14 & 4717.84-4721.84\\
Sm2 & 4791.5800 & 0.104 & -1.440 & (45) & 4791.28-4791.89 & 4789.59-4793.59\\
Sm2 & 4836.6600 & 0.104 & -2.190 & (45) & 4836.50-4836.75 & 4835.50-4837.80\\
Sm2 & 4836.6600 & 0.104 & -2.190 & (45) & 4836.50-4836.75 & 4835.50-4837.80\\
Sm2 & 4836.6600 & 0.104 & -2.190 & (45) & 4836.50-4836.75 & 4835.50-4837.80\\
Sm2 & 4836.6600 & 0.104 & -2.190 & (45) & 4836.50-4836.75 & 4835.50-4837.80\\
Sm2 & 4836.6600 & 0.104 & -2.190 & (45) & 4836.50-4836.75 & 4835.50-4837.80\\
Sm2 & 4836.6600 & 0.104 & -2.190 & (45) & 4836.50-4836.75 & 4835.50-4837.80\\
Sm2 & 4847.7600 & 0.659 & -0.890 & (45) & 4847.46-4848.06 & 4845.76-4849.76\\
Sm2 & 4854.3680 & 0.378 & -1.250 & (45) & 4854.20-4854.50 & 4853.20-4855.50\\
Sm2 & 4854.3680 & 0.378 & -1.250 & (45) & 4854.20-4854.50 & 4853.20-4855.50\\
Sm2 & 4854.3680 & 0.378 & -1.250 & (45) & 4854.20-4854.50 & 4853.20-4855.50\\
Sm2 & 4854.3680 & 0.378 & -1.250 & (45) & 4854.20-4854.50 & 4853.20-4855.50\\
Sm2 & 4854.3680 & 0.378 & -1.250 & (45) & 4854.20-4854.50 & 4853.20-4855.50\\
Sm2 & 4854.3680 & 0.378 & -1.250 & (45) & 4854.20-4854.50 & 4853.20-4855.50\\
Eu2 & 5818.7274 & 1.230 & -1.421 & (46) & 5818.40-5819.00 & 5816.73-5820.73\\
\hline
\multicolumn{7}{p{\textwidth}}{References: (1): \cite{1998PhRvA..57.1652Y} (2): \cite{1993AAS...99..179H} (3): \cite{NIST10} (4): \cite{GESMCHF} (5): \cite{2017A26A...598A.102P} (6): \cite{GESG12} (7): \cite{Kelleher} (8): \cite{K75} (9): \cite{GARZ|BL} (10): \cite{1993PhyS...48..297N} (11): \cite{Wang} (12): \cite{S} (13): \cite{SR} (14): \cite{LD} (15): \cite{2013ApJS..205...11L} (16): \cite{LGWSC} (17): \cite{NWL} (18): \cite{} (19): \cite{MFW} (20): \cite{BLNP} (21): \cite{WLSC} (22): \cite{2013ApJS..208...27W} (23): \cite{2014ApJS..215...20L} (24): \cite{SLS} (25): \cite{DLSSC} (26): \cite{FMW} (27): \cite{K08} (28): \cite{1982ApJ...260..395C} (29): \cite{2014ApJS..211...20W} (30): \cite{KR|1989ZPhyD..11..287C} (31): \cite{Grevesse} (32): \cite{1980AA....84..361B|1980ZPhyA.298..249K} (33): \cite{VGH} (34): \cite{K06} (35): \cite{BBEHL} (36): \cite{BGHL} (37): \cite{CB} (38): \cite{WBb} (39): \cite{WSL} (40): \cite{1992AA...255..457D} (41): \cite{LBS} (42): \cite{LSCI} (43): \cite{MC} (44): \cite{HLSC} (45): \cite{LD-HS} (46): \cite{LWHS}
}
